# Supplementary material for: A Four-Pronged Defense Against Byzantine Attacks in Federated Learning
Source: arXiv:2308.03331 source file (2023-08-07)
Supplement: Supplementary file 1 [file Appendix.tex]

\appendix{}
\section{More Experimental Result}

\begin{figure}[h]
\begin{center}
    \centering
    \includegraphics[width=0.9\textwidth]{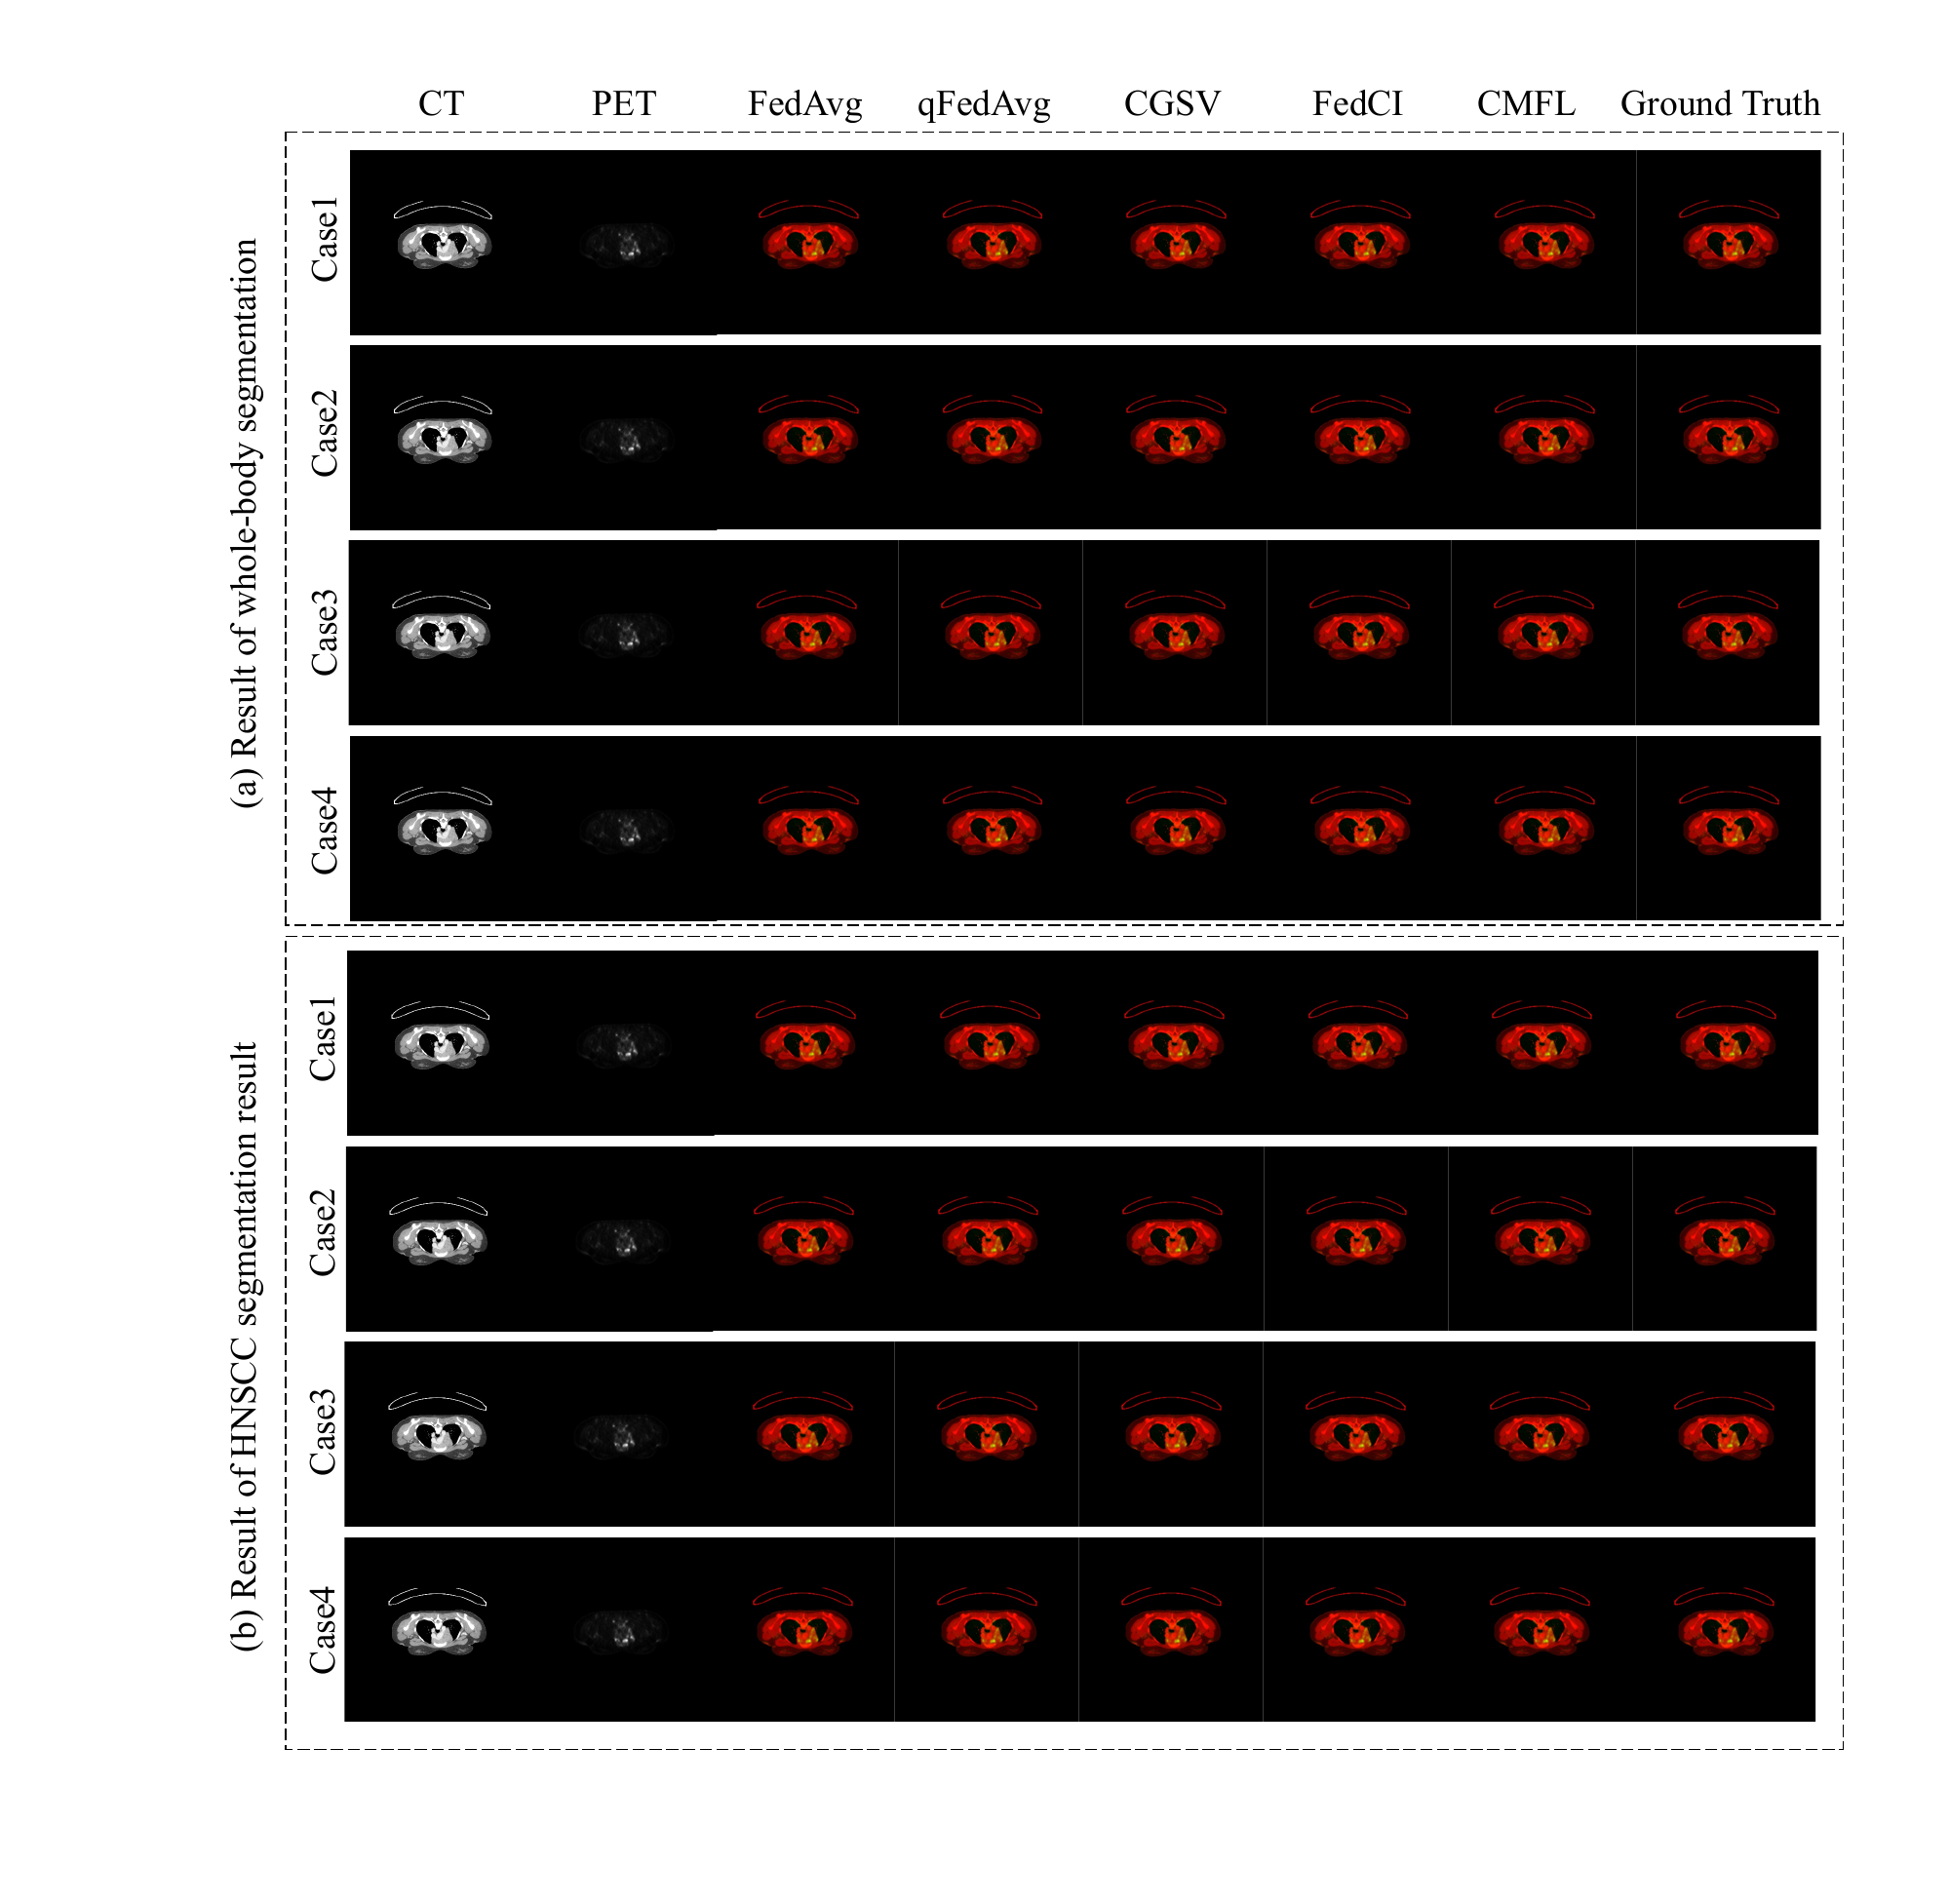}
\caption{\textbf{Visualization of image.}}
\end{center}
\end{figure}
